# Supplementary material for: Less is More: Mitigate Spurious Correlations for Open-Domain Dialogue Response Generation Models by Causal Discovery
Source: arXiv:2303.01962 source file (2023-03-02)
Supplement: Supplementary file 1 [file Appendix.tex]

\section{Appendix}
\label{sec:appendix}
